# Supplementary material for: 4DLangVGGT: 4D Language-Visual Geometry Grounded Transformer
Source: arXiv:2512.05060 source file (2025-12-04)
Supplement: Supplementary file 2 [file appendix_tab_joint2.tex]

\begin{table}[htbp!]
    \centering
    \setlength{\tabcolsep}{6pt}
    
    \caption{\textcolor{blue}{Comparison of \textbf{time-sensitive language queries} under single-model training on HyperNeRF. We report results from non-joint training and joint training variant.}}
    \label{tab:joint_time_sensitive}
    \vspace{-2mm}
    \resizebox{\linewidth}{!}{
    \begin{tabular}{lccccccccccc}
        \toprule
        \multirow{2}{*}{\centering Method} & \multirow{2}{*}{\centering Joint} &
        \multicolumn{2}{c}{\textbf{americano}} &
        \multicolumn{2}{c}{\textbf{chick-chicken}} &
        \multicolumn{2}{c}{\textbf{split-cookie}} &
        \multicolumn{2}{c}{\textbf{espresso}} &
        \multicolumn{2}{c}{\textbf{Average}}\\
        \cmidrule(lr){3-4} \cmidrule(lr){5-6} \cmidrule(lr){7-8} \cmidrule(lr){9-10} \cmidrule(lr){11-12}
        & & Acc & vIoU & Acc & vIoU & Acc & vIoU & Acc & vIoU & Acc & vIoU \\
        \midrule
        4DLangVGGT (Ours) & $\times$ & \textbf{90.03} & \textbf{67.77} & \textbf{97.81} & \textbf{93.44} & \textbf{95.76} & \textbf{84.02} & \textbf{82.86} & \textbf{52.06} & \textbf{91.44} & \textbf{74.74} \\
        \midrule
        4DLangVGGT (Ours, joint) & $\checkmark$ & 89.41 & 66.92 & 97.12 & 92.31 & 95.03 & 83.11 & 82.10 & 51.21 & 90.42 & 73.39 \\
        \bottomrule
    \end{tabular}
    }
\end{table}
